# Supplementary material for: Recall: Empowering Multimodal Embedding for Edge Devices
Source: arXiv:2409.15342 source file (2024-09-09)
Supplement: Supplementary file 1 [file sec-appendix.tex]

\newpage
\section*{Appendix}
\label{sec:appendix}

\begin{figure*}
    \centering
    \begin{minipage}[b]{0.4\textwidth}
        \centering
        \includegraphics[width=0.8\textwidth]{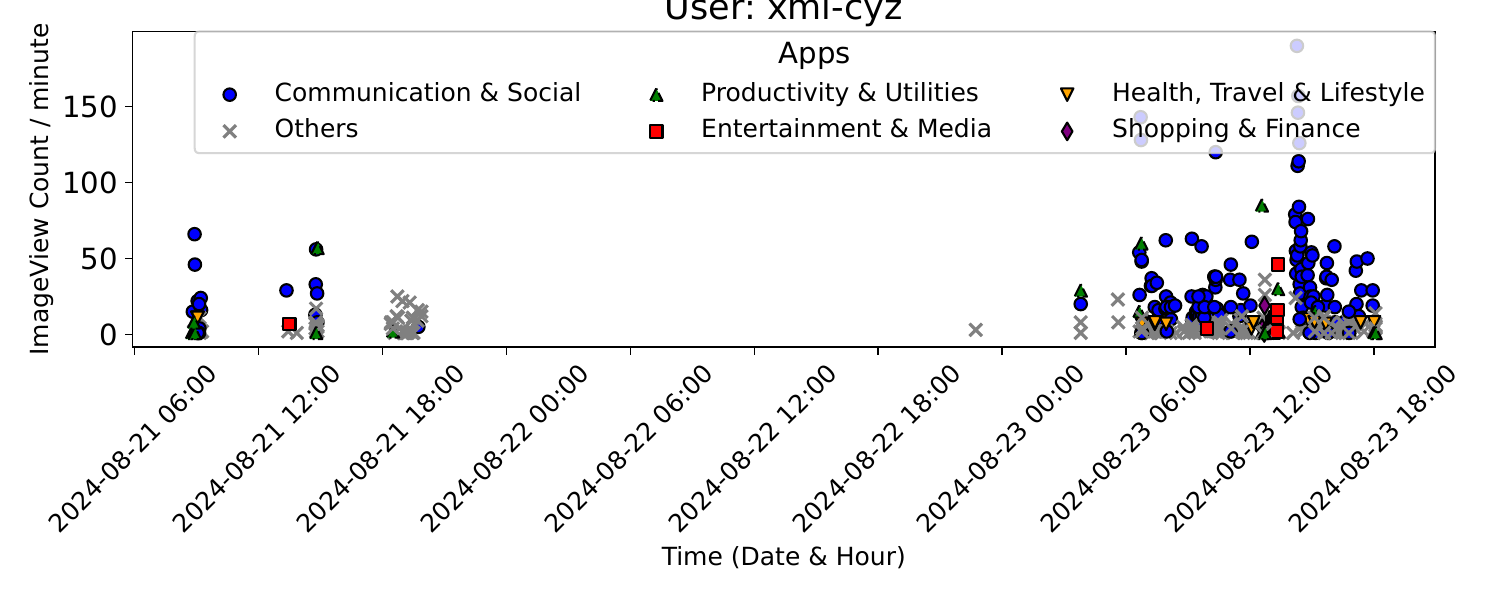}
        \subcaption{User 1: 55 years old} 
        % \label{fig:motivations-cost}
    \end{minipage}
    ~
    \begin{minipage}[b]{0.4\textwidth}
        \centering
        \includegraphics[width=0.8\textwidth]{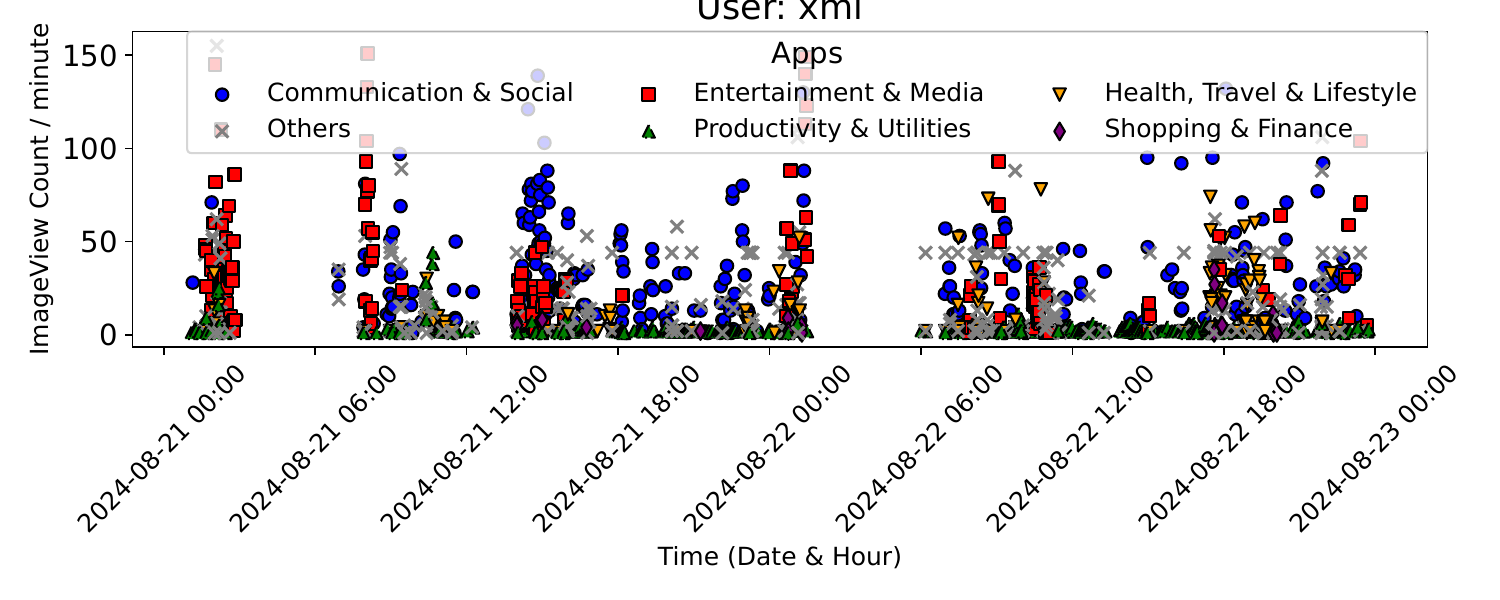}
        \subcaption{User 2: Man with} 
        % \label{fig:motivations-cost}
    \end{minipage}
    
    \begin{minipage}[b]{0.4\textwidth}
        \centering
        \includegraphics[width=0.8\textwidth]{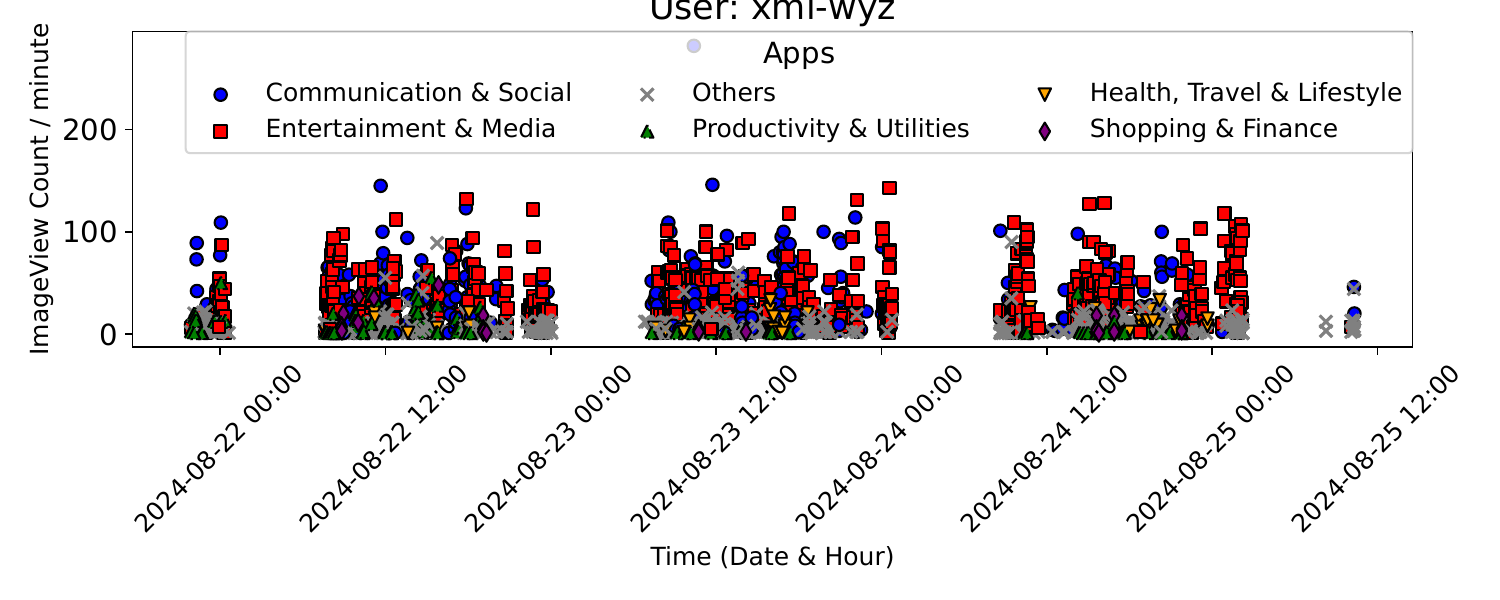}
        \subcaption{User 3: Yaozong Wu} 
        % \label{fig:motivations-cost}
    \end{minipage}
    ~
    \begin{minipage}[b]{0.4\textwidth}
        \centering
        \includegraphics[width=0.8\textwidth]{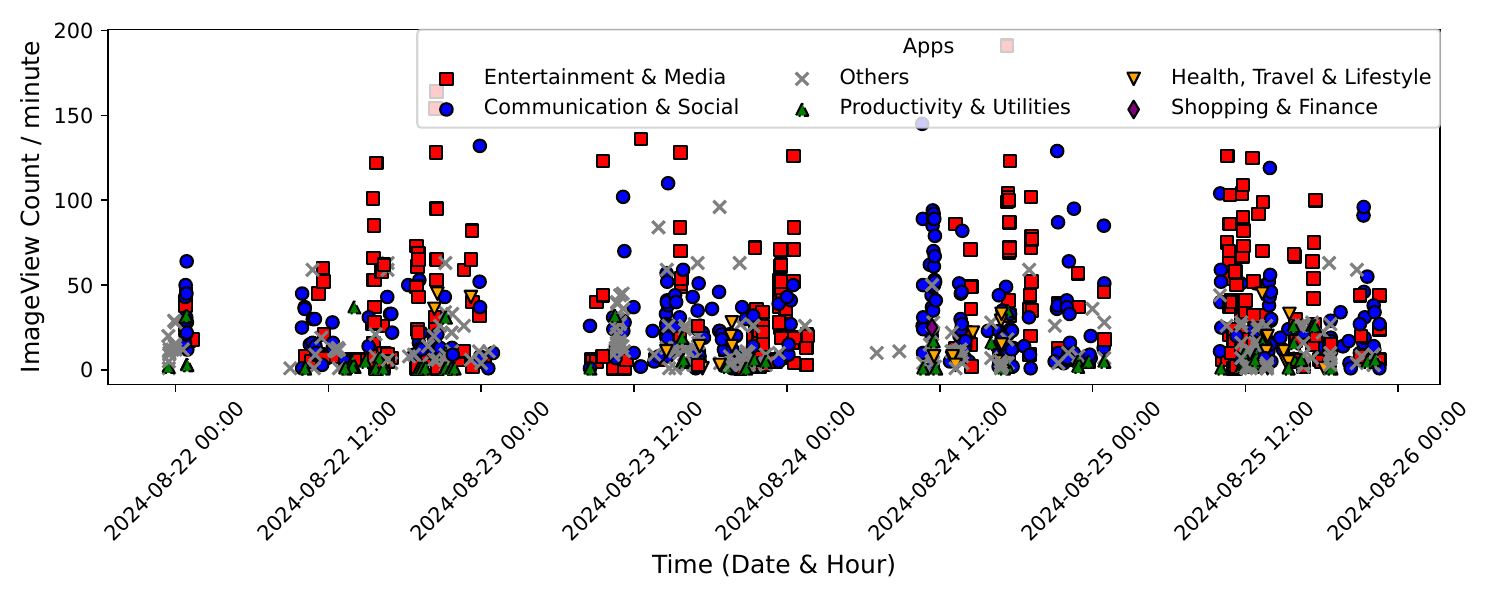}
        \subcaption{User 4: Weikai Xie} 
        % \label{fig:motivations-cost}
    \end{minipage}
    
    \begin{minipage}[b]{0.4\textwidth}
        \centering
        \includegraphics[width=0.8\textwidth]{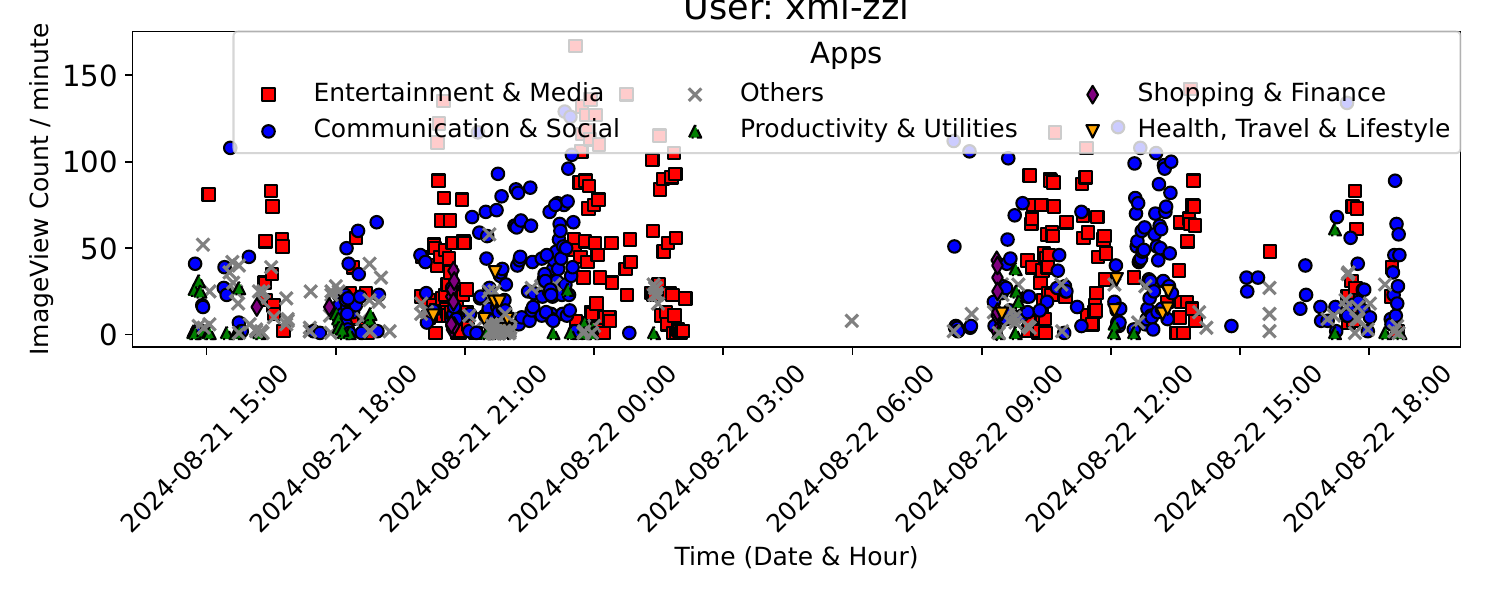}
        \subcaption{User 5: Zeling Zhang} 
        % \label{fig:motivations-cost}
    \end{minipage}
    ~
    \begin{minipage}[b]{0.4\textwidth}
        \centering
        \includegraphics[width=0.8\textwidth]{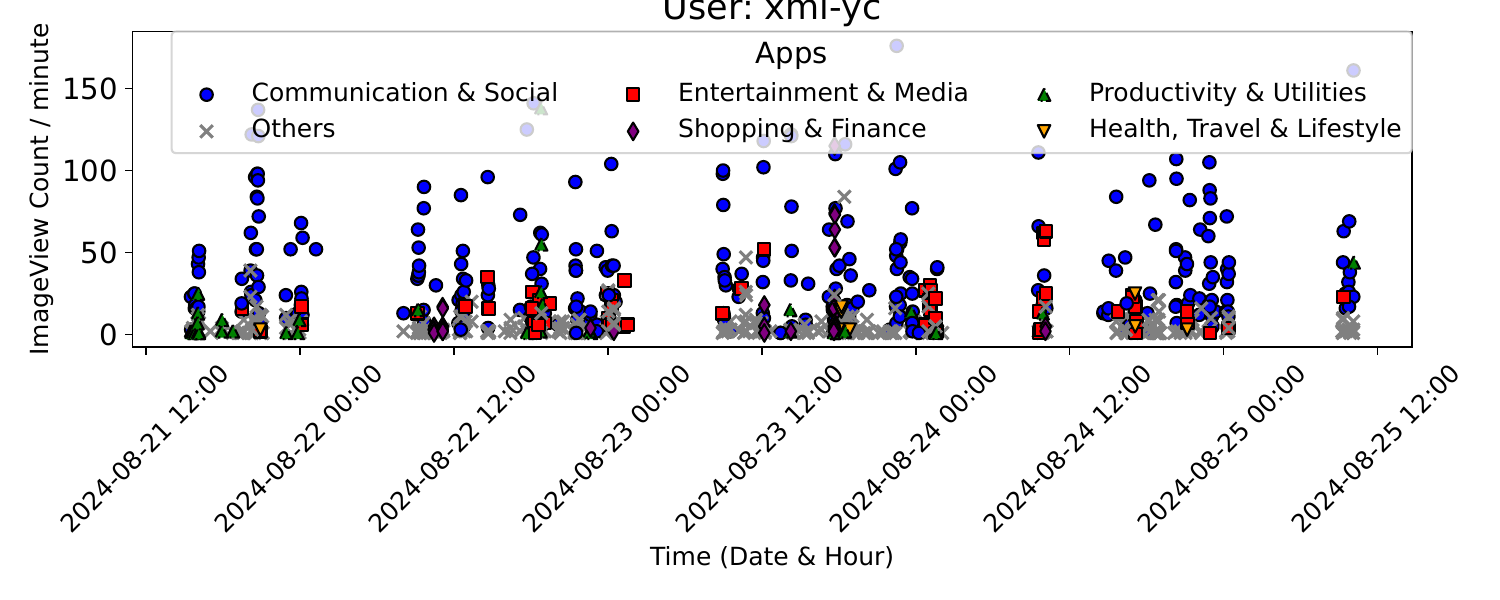}
        \subcaption{User 6: Cheng Yang} 
        % \label{fig:motivations-cost}
    \end{minipage}
    
    \caption{User study}
    % \vspace{-20pt}
    \label{fig:appendix-user-study}
\end{figure*}

    \begin{figure}[t]
    \begin{minipage}[b]{0.23\textwidth}
        \centering
        \includegraphics[width=0.8\textwidth]{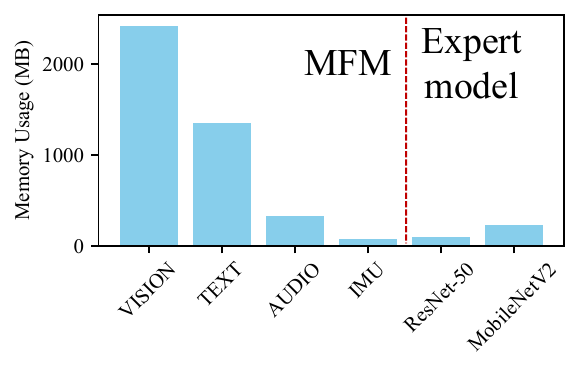}
	 \vspace{-10pt}
	\subcaption{Memory} 
	% \vspace{-15pt}
	\label{fig:motivations-loading}
    \end{minipage}
    ~
    \begin{minipage}[b]{0.23\textwidth}
        \centering
        \includegraphics[width=0.9\textwidth]{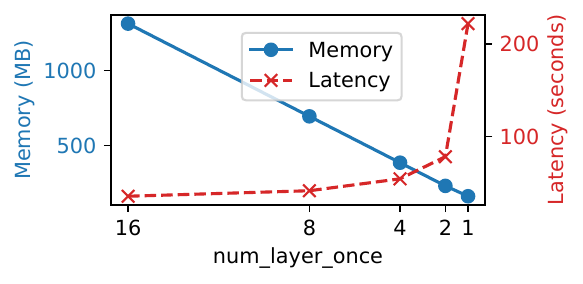}
	%  \vspace{-10pt}
	\subcaption{Layer-wise encoding} 
	% \vspace{-15pt}
	\label{fig:motivations-loading}
    \end{minipage}
	% \vspace{-10pt}    
    \caption{Memory issue. (a) It is highly likely to be a victim to OS memory killer; (b) Merits and drawbacks of layer-by-layer encoding. BS=1, \# of encoded figures=50..}
    % \vspace{-20pt}
    \label{fig:motivations-memory}
\end{figure}

% \begin{figure}[t]
% 	\centering
% 	 \includegraphics[width=0.3\textwidth]{figs/motivation-loading.pdf}
% 	%  \vspace{-10pt}
% 	\caption{Merits and drawbacks of layer-by-layer encoding. BS=1, \# of encoded figures=50. } 
% 	% \vspace{-15pt}
% 	\label{fig:motivations-loading}
% \end{figure}
\begin{figure}[t]
	\centering
	 \includegraphics[width=0.45\textwidth]{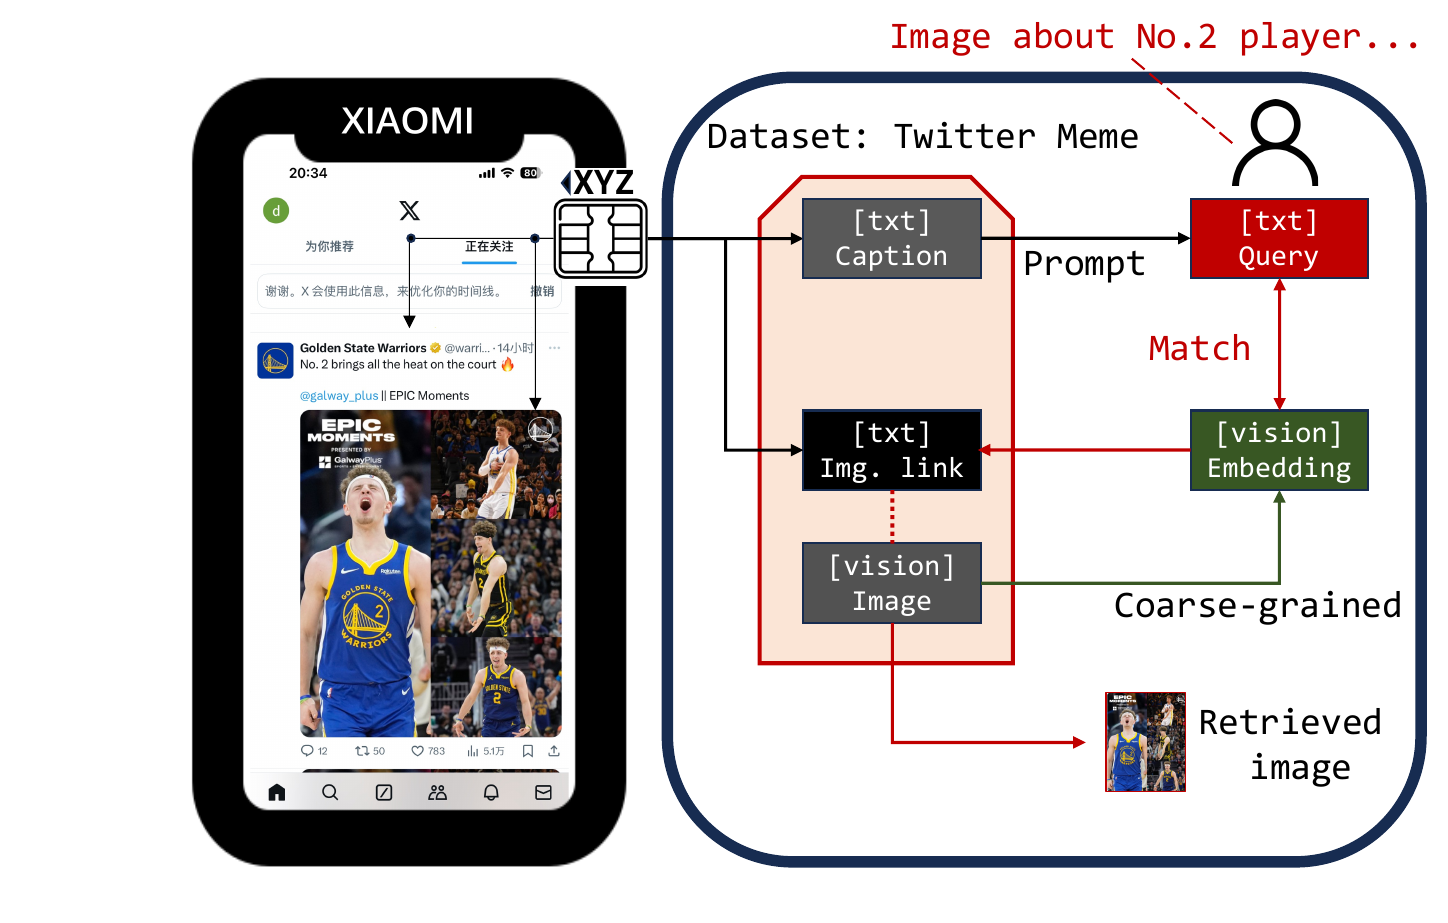}
	%  \vspace{-10pt}
	\caption{Case study: Daily personal application retrieval.
	\cdq{Could move to Appendix.}
	} 
	% \vspace{-15pt}
	\label{fig:eval-case}
\end{figure}
\subsection{User study on viewed images}
We collect viewed images of daily mobile applications from 8 volunteers, ranging from 20 to 52 years old.
Uiautomator was executed at the backward to dump daily android UI page (stored in xml file format) for final analysis.

{\scriptsize
\begin{verbatim}
    <?xml version="1.0" encoding="UTF-8" standalone="yes"?>
    <hierarchy rotation="0">
        <node>
            ...
            <node 
                index="1" 
                text="Brita Kettle..."
                resource-id="com.xingin.xhs:id/cy7"
                class="android.widget.ImageView"
                package="com.xingin.xhs"
                content-desc="product photo"
                checkable="false"
                checked="false"
                clickable="true"
                enabled="true"
                focusable="true"
                focused="false"
                scrollable="false"
                long-clickable="false"
                password="false"
                selected="false"
                bounds="[0,114][78,213]"
            />
            ...
        </node>
    </hierarchy>
    \end{verbatim}
}

Top-10 applications generating the most viewed images are displayed to show the user trace.

The `ImageView' elements are detected to monitor whether there is the new figures.
% We then analyze 
Relevant images and their description are saved in storage for future retrieval.

Each imageview xml element group is hashed to only include newly appeared images.
resource-id can help to index the raw images to excluding icons and other small system UIs.

\subsection{Memory issue and loading latency}

\textbf{Memory issue.}
Apart from slow inference, memory is another killer that makes it hard to deploy the model on mobile devices and hold the model persistently.
For example, the ImageBind model weights are around 1.5GB, which is too large for mobile devices.
This causes the application to be easily killed by the OS due to memory pressure.
as shown in Figure~\ref{fig:motivations-memory}.
Storing the complete model weights for each modality is memory-intensive.
For example, the ImageBind model weights are around 1.5GB, which is too large for mobile devices.
This causes the application to be easily killed by the OS due to memory pressure.
Even after the model is quantized to INT4, it still occupies more than 0.2GB of memory for the weights, not to mention the intermediate activations.
This causes the application to be easily killed by the OS due to memory pressure.

% \paragraph{Observation-4: Layerwise Model Execution Can Save Memory but Significantly Increase Encoding Time}
% Layerwise model Execution Can Save Memory but Significantly Increase Encoding Time
\textbf{Loading latency of layerwise inference.}
One common solution is to load the model layer by layer and sequentially remove the weights from the memory after finishing relevant operations.
It can save memory by up to \cdq{10}$\times$ for executing MFM inference.
However, the loading latency for each transformer block is around 0.27s, which is 7$\times$ larger than the encoding time of each block (around 0.04s for one image).
This leads to a significant increase in the encoding time, as shown in Figure~\ref{fig:motivations-loading}.

\cdq{repeated to show figures.}
\textbf{Loading latency of layerwise inference.}
One common solution is to load the model layer by layer and sequentially remove the weights from the memory after finishing relevant operations.
It can save memory by up to \cdq{10}$\times$ for executing MFM inference.
However, the loading latency for each transformer block is around 0.27s, which is 7$\times$ larger than the encoding time of each block (around 0.04s for one image).
This leads to a significant increase in the encoding time, as shown in Figure~\ref{fig:motivations-loading}.

\textbf{Loading latency of layerwise inference.}
One common solution is to load the model layer by layer and sequentially remove the weights from the memory after finishing relevant operations.
It can save memory by up to \cdq{10}$\times$ for executing MFM inference.
However, the loading latency for each transformer block is around 0.27s, which is 7$\times$ larger than the encoding time of each block (around 0.04s for one image).
This leads to a significant increase in the encoding time, as shown in Figure~\ref{fig:motivations-loading}.

\textbf{Loading latency of layerwise inference.}
One common solution is to load the model layer by layer and sequentially remove the weights from the memory after finishing relevant operations.
It can save memory by up to \cdq{10}$\times$ for executing MFM inference.
However, the loading latency for each transformer block is around 0.27s, which is 7$\times$ larger than the encoding time of each block (around 0.04s for one image).
This leads to a significant increase in the encoding time, as shown in Figure~\ref{fig:motivations-loading}.

\textbf{Loading latency of layerwise inference.}
One common solution is to load the model layer by layer and sequentially remove the weights from the memory after finishing relevant operations.
It can save memory by up to \cdq{10}$\times$ for executing MFM inference.
However, the loading latency for each transformer block is around 0.27s, which is 7$\times$ larger than the encoding time of each block (around 0.04s for one image).
This leads to a significant increase in the encoding time, as shown in Figure~\ref{fig:motivations-loading}.

\textbf{Loading latency of layerwise inference.}
One common solution is to load the model layer by layer and sequentially remove the weights from the memory after finishing relevant operations.
It can save memory by up to \cdq{10}$\times$ for executing MFM inference.
However, the loading latency for each transformer block is around 0.27s, which is 7$\times$ larger than the encoding time of each block (around 0.04s for one image).
This leads to a significant increase in the encoding time, as shown in Figure~\ref{fig:motivations-loading}.

\textbf{Loading latency of layerwise inference.}
One common solution is to load the model layer by layer and sequentially remove the weights from the memory after finishing relevant operations.
It can save memory by up to \cdq{10}$\times$ for executing MFM inference.
However, the loading latency for each transformer block is around 0.27s, which is 7$\times$ larger than the encoding time of each block (around 0.04s for one image).
This leads to a significant increase in the encoding time, as shown in Figure~\ref{fig:motivations-loading}.

\textbf{Loading latency of layerwise inference.}
One common solution is to load the model layer by layer and sequentially remove the weights from the memory after finishing relevant operations.
It can save memory by up to \cdq{10}$\times$ for executing MFM inference.
However, the loading latency for each transformer block is around 0.27s, which is 7$\times$ larger than the encoding time of each block (around 0.04s for one image).
This leads to a significant increase in the encoding time, as shown in Figure~\ref{fig:motivations-loading}.

\subsection{Case Study: Twitter Meme Retrieval}

To reveal the practicality of \sys in real world scenarios, we collected daily surfing images and relevant captions from Twitter memes from the Internet as shown in Figure~\ref{fig:eval-case}.
The data were filtered by end users to avoid privacy issues.
The filtered dataset comprises 1,000 images and 1,000 relevant captions, denoted as the \texttt{MEME} dataset for numerical accuracy evaluation.
These figures are not stored locally; only their links are saved to conserve storage.
The tested device is a commodity mobile phone with 4GB memory and a 2GHz CPU.
The inference engine used is the open-sourced multimodal inference engine mllm~\cite{mllm24}.
