# Supplementary material for: Recall: Empowering Multimodal Embedding for Edge Devices
Source: arXiv:2409.15342 source file (2024-09-09)
Supplement: Supplementary file 2 [file fig-appendix-trace.tex]

\begin{figure*}
    \centering
    \begin{minipage}[b]{0.4\textwidth}
        \centering
        \includegraphics[width=0.8\textwidth]{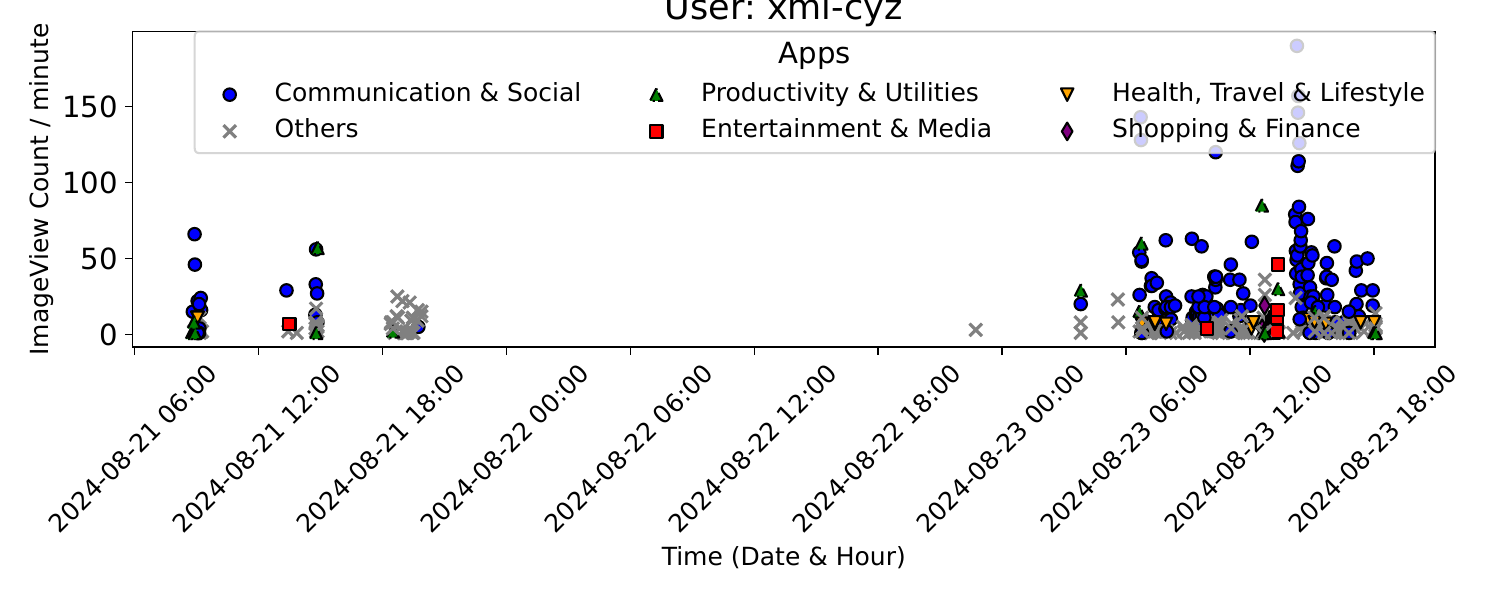}
        \subcaption{User 1: 55 years old} 
        % \label{fig:motivations-cost}
    \end{minipage}
    ~
    \begin{minipage}[b]{0.4\textwidth}
        \centering
        \includegraphics[width=0.8\textwidth]{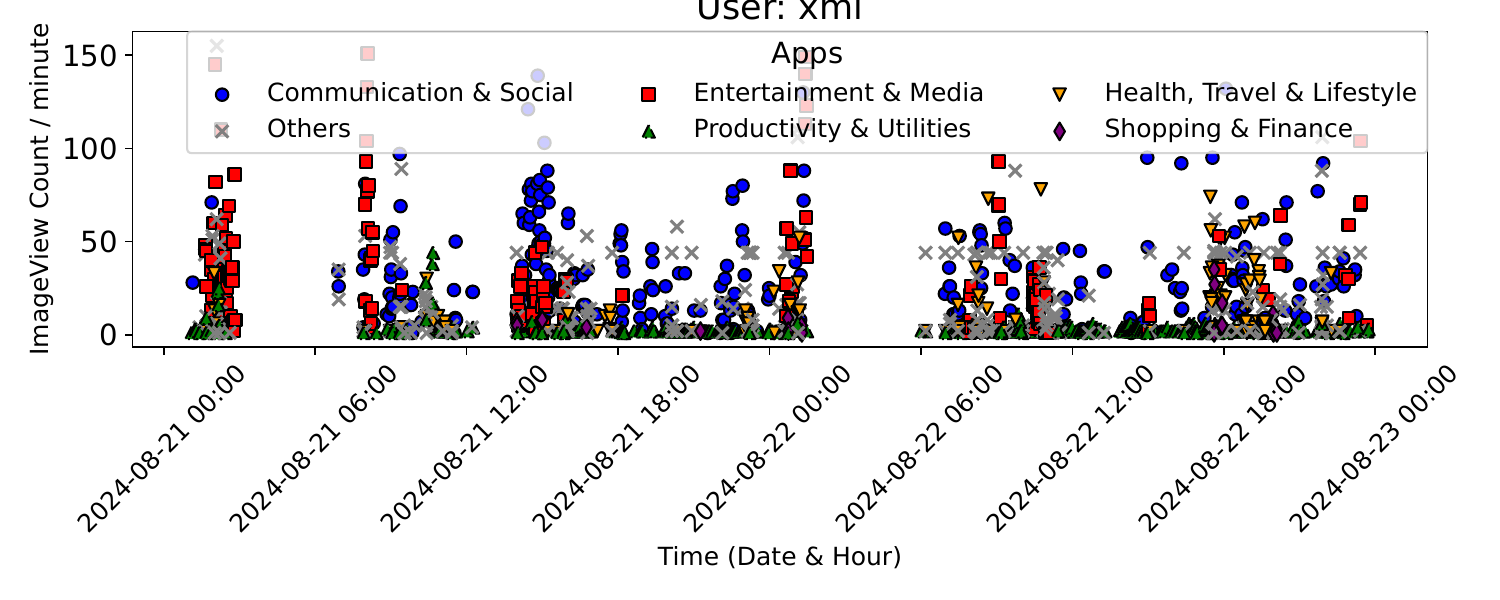}
        \subcaption{User 2: Man with} 
        % \label{fig:motivations-cost}
    \end{minipage}
    
    \begin{minipage}[b]{0.4\textwidth}
        \centering
        \includegraphics[width=0.8\textwidth]{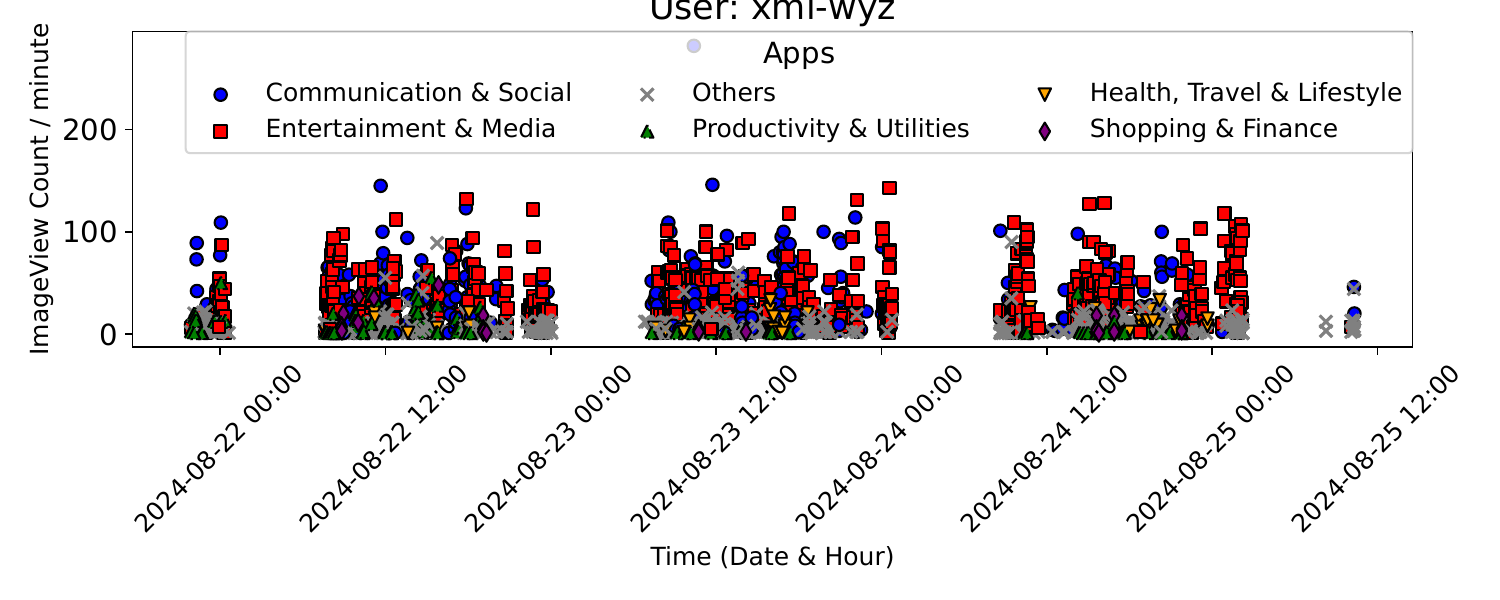}
        \subcaption{User 3: Yaozong Wu} 
        % \label{fig:motivations-cost}
    \end{minipage}
    ~
    \begin{minipage}[b]{0.4\textwidth}
        \centering
        \includegraphics[width=0.8\textwidth]{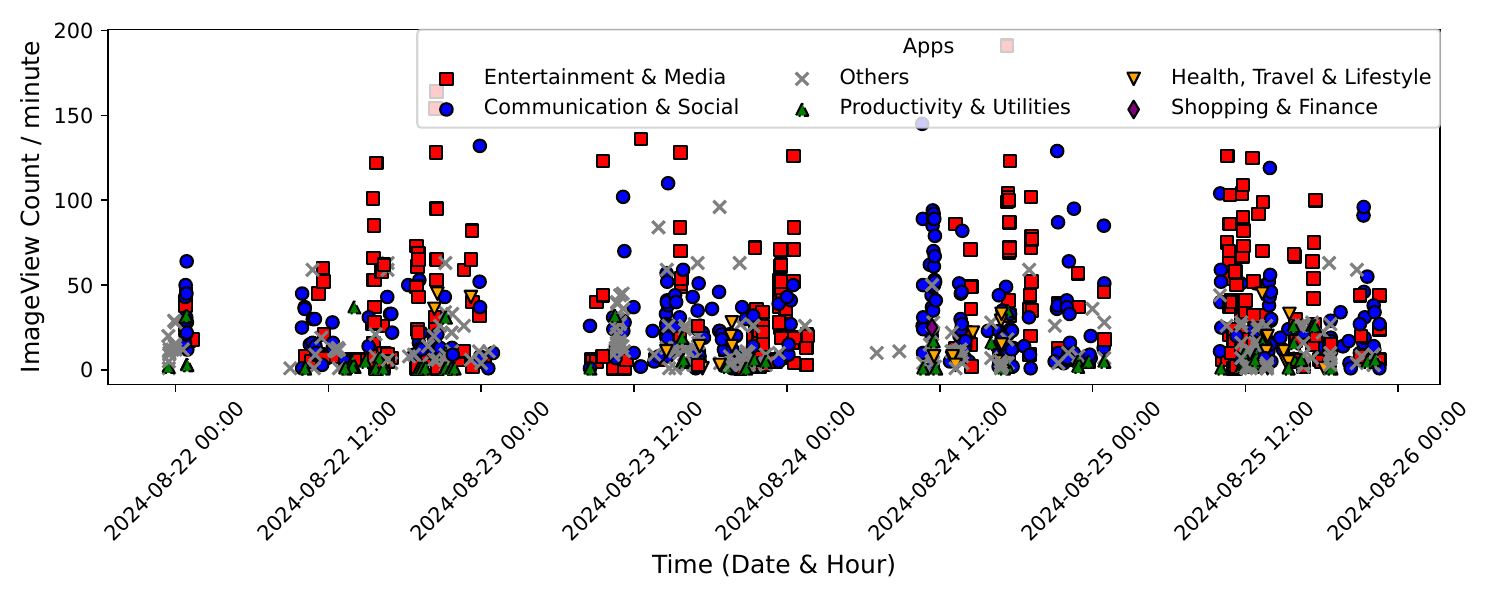}
        \subcaption{User 4: Weikai Xie} 
        % \label{fig:motivations-cost}
    \end{minipage}
    
    \begin{minipage}[b]{0.4\textwidth}
        \centering
        \includegraphics[width=0.8\textwidth]{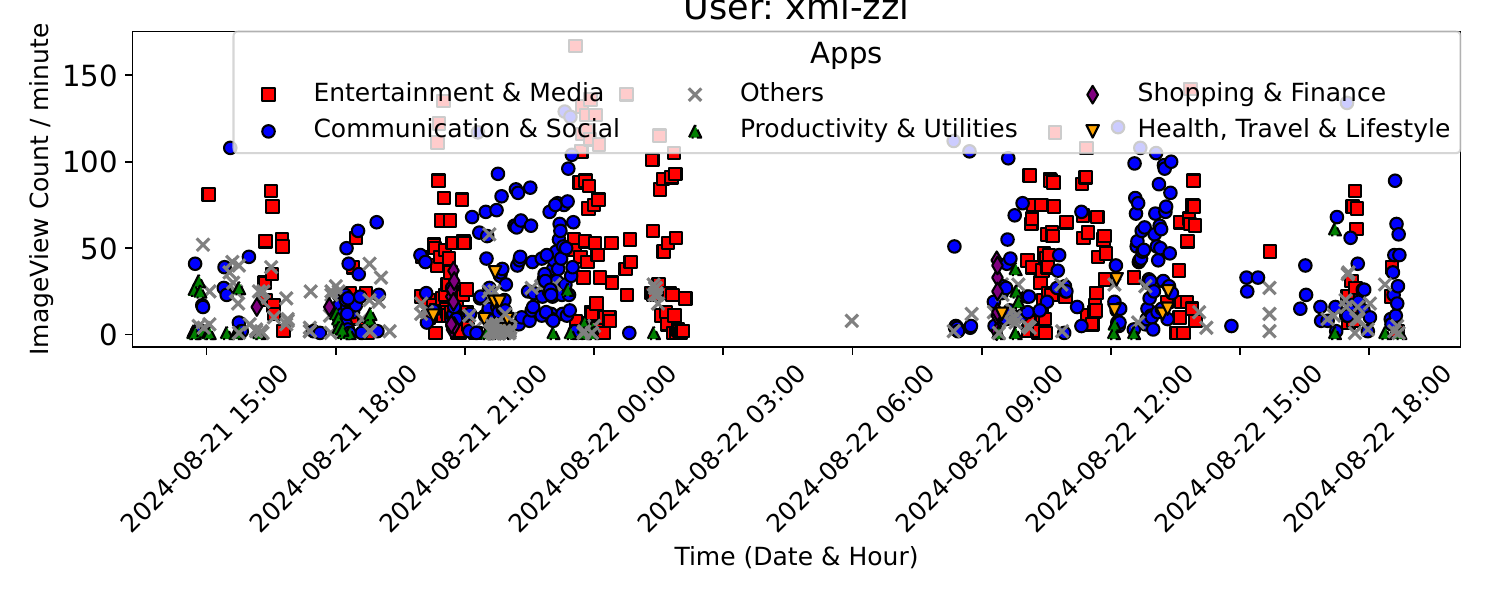}
        \subcaption{User 5: Zeling Zhang} 
        % \label{fig:motivations-cost}
    \end{minipage}
    ~
    \begin{minipage}[b]{0.4\textwidth}
        \centering
        \includegraphics[width=0.8\textwidth]{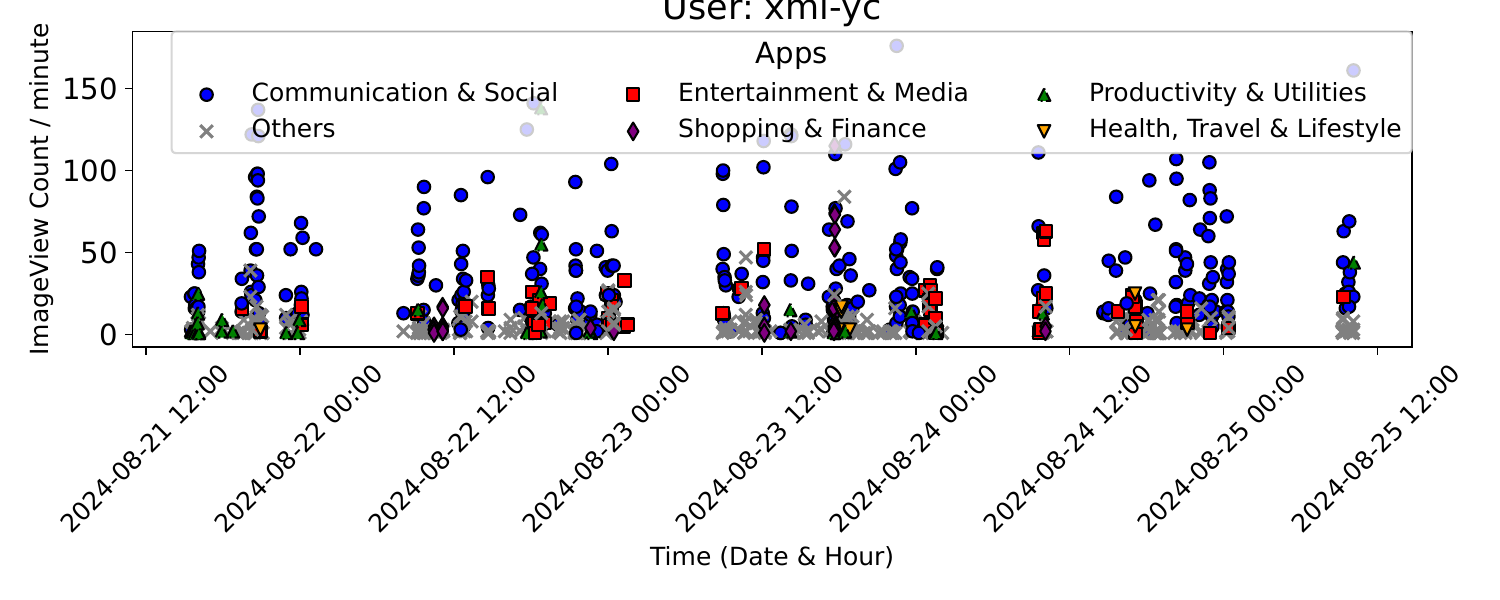}
        \subcaption{User 6: Cheng Yang} 
        % \label{fig:motivations-cost}
    \end{minipage}
    
    \caption{User study}
    % \vspace{-20pt}
    \label{fig:appendix-user-study}
\end{figure*}
